# Supplementary material for: Efficient Algorithms with Asymmetric Read and Write Costs
Source: arXiv:1511.01038 source file (2016-08-28)
Supplement: Supplementary file 1 [file appendix-.tex]

\section{Motivation from~\cite{BFGGS15}}

Further motivation for the asymmetry between reads and write costs in
emerging memory technologies was provided in~\cite{BFGGS15}.  As a
convenience to the reviewer, in this appendix we repeat a suitable
excerpt from that paper.

``While DRAM stores data in capacitors that
typically require refreshing every few milliseconds,
and hence must be continuously powered, emerging NVM
technologies store data as ``states'' of the given material that
require no external power to retain.  Energy is required only to read
the cell or change its value (i.e., its state).  While there is no
significant cost difference between reading and writing DRAM (each
DRAM read of a location not currently buffered requires a write of
the DRAM row being evicted, and hence is also a write),
emerging NVMs such as Phase-Change Memory (PCM), Spin-Torque
Transfer Magnetic RAM (STT-RAM), and Memristor-based Resistive RAM
(ReRAM) each incur significantly higher cost for writing than reading.
This large gap seems fundamental to the technologies themselves: to
change the physical state of a material requires relatively
significant energy for a sufficient duration, whereas reading the
current state can be done quickly and, to ensure the state is left
unchanged, with low energy.  An STT-RAM cell, for example, can be read
in 0.14 $ns$ but uses a 10 $ns$ writing pulse duration, using roughly
$10^{-15}$ joules to read versus $10^{-12}$ joules to
write~\cite{Dong08} (these are the raw numbers at the materials
level).  A Memristor ReRAM cell uses a 100 $ns$ write pulse duration, and
an 8MB Memrister ReRAM chip is projected to have reads with 1.7 $ns$
latency and 0.2 $nJ$ energy versus writes with 200 $ns$ latency and 25 $nJ$
energy~\cite{Xu11}---over two orders of magnitude differences in latency
and energy.  PCM is the most mature of the three technologies, and
early generations are already available as I/O devices.  A recent
paper~\cite{Kim14} reported 6.7 $\mu s$ latency for a 4KB read and
128 $\mu s$ latency for a 4KB write.  Another reported that the
sector I/O latency and bandwidth for random 512B writes was a factor
of 15 worse than for reads~\cite{ibm-pcm14b}.  As a future memory/cache
replacement, a 512Mb PCM memory chip is projected to have 16 $ns$ byte
reads versus 416 $ns$ byte writes, and writes to a 16MB PCM L3 cache
are projected to be up to 40 times slower and use 17 times more energy
than reads~\cite{Dong09}.  While these numbers are speculative and subject
to change as the new technologies emerge over time, there seems to be
sufficient evidence that writes will be considerably more costly than
reads in these NVMs.''

Note that, unlike SSDs and earlier versions of phase-change memmory products,
these emerging memory products will sit on the processor's memory bus and be
accessed at byte granularity via loads and stores (like DRAM).  Thus, the
time and energy for reading can be roughly on par with DRAM, and depends
primarily on the properties of the technology itself relative to DRAM.

\input{MST}

\section{Longest Common Subsequence: Further Results}\label{sec:LCS-app}

\input{LCS-app}

%\section{Single-Source Shortest Path: Further Details}

%\phil{Move parts of the SSSP section here that don't fit, e.g., the pseudocode.}

\input{floyd-warshall.tex}
